# Supplementary material for: Tabling as a Library with Delimited Control
Source: arXiv:1507.08087 source file (2015-07-29)
Supplement: Supplementary file 1 [file appendixExampleResolutionTree.tex]

Figure~\ref{fig:runningExampleResolutionTree} shows the full resolution tree for our running example. For reasons of clarity, we have not depicted the completion phase in full detail.

\begin{figure*}
  \begin{center}
  \includestandalone[width=0.9\textwidth]{tikzQueryDiagram/main}
  \end{center}
  \caption{Resolution tree for our running example.\label{fig:runningExampleResolutionTree}}
\end{figure*}
